# Supplementary material for: KGLiDS: A Platform for Semantic Abstraction, Linking, and Automation of Data Science
Source: arXiv:2303.02204 source file (2024-06-12)
Supplement: Supplementary file 1 [file supplementary_material.tex]

\clearpage
\appendix

\section*{Supplementary Materials}

\section*{F1-Scores of Table Relatedness}

\begin{figure}[h]
  \centering
  \subfloat[a][\texttt{Smaller Real}]{\includegraphics[width=\columnwidth]{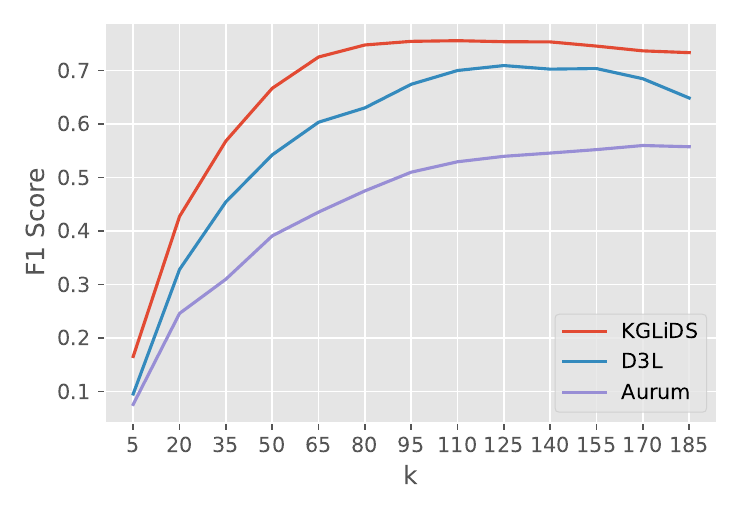}  \label{fig:experiment_f1_smaller_real}} \\
  \subfloat[b][\texttt{Synthetic}]{\includegraphics[width=\columnwidth]{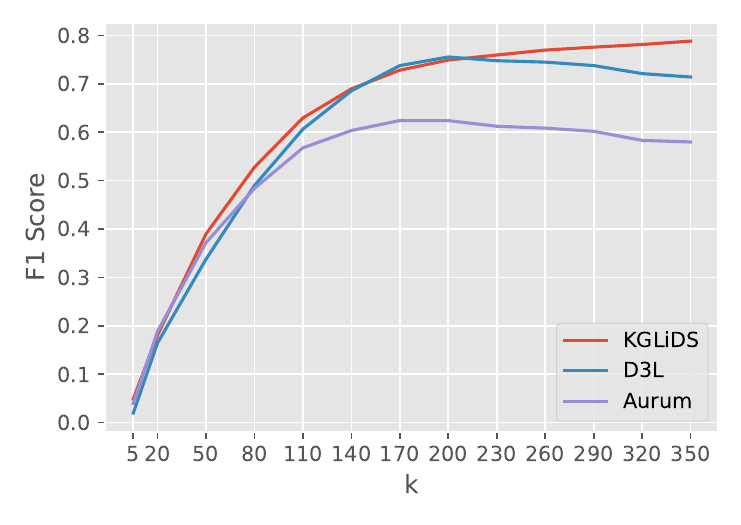}  \label{fig:experiment_f1_synthetic}}
  
  \caption{Average F1-Score of table relatedness for {\sysname}, $D^3L$, and Aurum on \texttt{Smaller Real} and \texttt{Synthetic} datasets for different values of $k$.}
  
  \label{fig:experiment_f1}
  
\end{figure}

\section*{SPARQL Queries for Query-Based APIs}

In this section, we provide the corresponding SPARQL queries to the ones mentioned in \autoref{sec:use_cases}. All the following queries using these prefixes:

\begin{lstlisting}
PREFIX kglids: <http://kglids.org/>
PREFIX data: <http://kglids.org/data/>
PREFIX pipeline: <http://kglids.org/pipeline/>
\end{lstlisting}

\subsection*{Finding joinable/unionable tables to a given one}

\begin{lstlisting}
SELECT distinct ?similar_table
WHERE {
    ?col_in_target_table kglids:isPartOf <http://kglids.org/datasnaek.youtube-new/dataResource/CAvideos.csv> . #example table
    ?col_in_target_table data:semanticSimilarity ?col_in_similar_table . # data:pkfk for joinable
    ?col_in_similar_table kglids:isPartOf ?similar_table
}
\end{lstlisting}

\subsection*{Finding a common schema between two tables}

\begin{lstlisting}
SELECT DISTINCT ?col_in_table_1 ?col_in_table_2
WHERE {
    ?col_in_table_1 kglids:isPartOf <http://kglids.org/datasnaek.youtube-new/dataResource/CAvideos.csv> . #example table
    ?col_in_table_2 kglids:isPartOf <http://kglids.org/kaggle/shivamb.netflix-shows/dataResource/netflix_titles.csv> .  # example table
    ?col_in_table_1 data:semanticSimilarity ?col_in_table_2
}
\end{lstlisting}

\subsection*{Finding whether two tables have a join path}

\begin{lstlisting}
ASK
{
 <http://kglids.org/datasnaek.youtube-new/dataResource/CAvideos.csv> 
   data:isJoinableWith+ 
   <http://kglids.org/kaggle/shivamb.netflix-shows/dataResource/netflix_titles.csv> .
}
\end{lstlisting}

\subsection*{Fining pipelines that use a particular module (e.g.RandomForestClassifier)}

\begin{lstlisting}
SELECT DISTINCT ?pipeline
WHERE {
    GRAPH ?pipeline {
        ?statement a pipeline:statement .
        ?statement pipeline:callsLibrary <http://kglids.org/pipeline/library/sklearn/ensemble/RandomForestClassifier>
    }
}
\end{lstlisting}

\subsection*{Discovering common classifiers used with a certain feature selection model}

\begin{lstlisting}
SELECT DISTINCT ?classifier (COUNT(?classifier) AS ?classifier_count)
WHERE {
    GRAPH ?pipeline {
        ?statement_feature_statement a pipeline:statement .
        ?statement_feature_statement pipeline:callsLibrary <http://kglids.org/pipeline/library/sklearn/feature_selection/SelectKBest> .
        ?statement_classifier a pipeline:statement .
        ?statement_classifier pipeline:callsLibrary ?classifier` .
        FILTER(REGEX(STR(?classifier), "classifier", "i"))
    }
}
GROUP BY ?classifier
ORDER BY DESC(?classifier_count)
\end{lstlisting}

\subsection*{Finding the most used sub-packages for a certain library}

\begin{lstlisting}
SELECT ?subpackage (COUNT(?subpackage) AS ?subpackage_count)
WHERE {
    ?subpackage kglids:isPartOf+ <http://kglids.org/pipeline/library/pandas> .
    GRAPH ?pipeline {
        ?statement a pipeline:statement .
        ?statement pipeline:callsLibrary ?subpackage
    }
}
GROUP BY ?subpackage
ORDER BY DESC(?subpackage_count)
\end{lstlisting}

\subsection*{Finding short or long pipelines}

\begin{lstlisting}
SELECT ?pipeline (COUNT(?statement) AS ?statement_count)
WHERE {
    GRAPH ?pipeline {
        ?statement a pipeline:statement .
    }
}
GROUP BY ?pipeline ?statement
HAVING (?statement_count < 100) # short pipelines
ORDER BY ?statement_count
\end{lstlisting}

\subsection*{Finding the top-k used columns (i.e. features) in a specific table}

\begin{lstlisting}
SELECT ?column (COUNT(?column_reading_steatement) AS ?column_reads)
WHERE {
    ?column a data:column .
    ?column kglids:isPartOf <http://kglids.org/datasnaek.youtube-new/dataResource/CAvideos.csv> # example table
    GRAPH ?pipeline {
        ?column_reading_steatement a pipeline:statement .
        ?column_reading_steatement pipeline:reads ?column
    }
}
GROUP BY ?column
ORDER BY DESC(?column_reads)
LIMIT 3
\end{lstlisting}

\subsection*{Finding the most common preprocessings on a specific column}

\begin{lstlisting}
SELECT ?preprocessing_module (COUNT(?statement) AS ?module_use)
WHERE {
    ?preprocessing_module kglids:isPartOf+ <http://kglids.org/pipeline/library/sklearn/preprocessing>
    GRAPH ?pipeline {
        ?statement a pipeline:statement .
        ?statement pipeline:callsLibrary ?preprocessing_module .
        ?statement pipeline:reads <http://kglids.org/kaggle/shivamb.netflix-shows/dataResource/netflix_titles.csv/titles> # example column
    }
}
GROUP BY ?preprocessing_module ?statement
ORDER BY DESC(?module_use)
\end{lstlisting}

\subsection*{ Finding common parameter values of a specific classifier (e.g.SVM) on a specific dataset}

\begin{lstlisting}
SELECT ?param_name ?param_value (COUNT(?param_value) AS ?value_count)
WHERE {
    GRAPH ?pipeline {
        ?svm_statement a pipeline:statement .
        ?svm_statement pipeline:callsLibrary <http://kglids.org/pipeline/library/sklearn/svm/SVC> .
        <<?svm_statement pipeline:hasParameter ?param_name>> pipeline:parameterValue ?param_value
    }
}
GROUP BY ?param_name ?param_value
ORDER BY DESC(?value_count)
\end{lstlisting}
